# Supplementary material for: Real-Time LSM-Trees for HTAP Workloads
Source: arXiv:2101.06801 source file (2022-07-15)
Supplement: Supplementary file 1 [file appendix.tex]

\textbf{Estimating $E^G_i$ and $E^g_i$:} 
%As seen in Section \ref{sec:cost-analysis}, value of $E^G_i$ and $E^g_i$ depends on the operation's projection $R$ and CG configuration of the LSM Tree. In rest of the section we discuss how $E^G_i$ and $E^g_i$ can be estimated as a function of workload projection and CG configuration, and how Equation \ref{eq:cost} can be used to find best CG configuration.
We estimate the values of $E^G_i$ and $E^g_i$, similar to how cardinalities are estimated in query optimization \cite{cow-book}: i.e., (1) either by collecting statistics about the workload, or, (2) in the case where statistics are not available, we rely on certain assumptions about the workload. Similar to cardinality estimation, our approach does not guarantee finding the optimal CG layout due to the lack of precise statistics, but we aim to avoid bad CG configurations and find good ones. We discuss the above two scenarios and explain how good CG configurations can be found.

%The projection $R$ could in principle be different for each operation of the workload; and a complex workload analysis will be required to plug-in those values in the optimization function. On the other hand, it can be estimated based on certain assumptions about the workload or using average or median statistics about the workload operations. Note that the proximity of the optimal column-group configuration discovered by the optimization function to the "true-best" column-group configuration (which is unknown) will depend on how accurately we estimate $E^G_i$ and $E^g_i$.  We show two example scenarios of how to estimate these values.

\textit{Scenario 1:} In this scenario we estimate $E^G_i$ and $E^g_i$ based on the following assumptions about the workload:
\begin{enumerate}
    \item We assume that on average the \textit{read} and \textit{update} operation's projection is wide enough that it needs to fetch values from each column-group.
    \item The \textit{scan} operation has narrow projection such that one column-group is enough to answer the query.
    \item \textit{Read} and \textit{update} operations are restricted to smaller levels (i.e. recent data).
\end{enumerate}
These assumptions are in-line with HTAP workload characteristics \cite{htapSurvey,gartnerHTAP}. With these assumptions, for \textit{read} operations, we have value $E^g_i = g_i$, (because read operation at level $i$ spans all the CGs at level $i$), for scan operations we have $E^G_i = c/g_i$, (because scan needs only one CG, and average size of CG can be estimated to be $c/g_i$), and for update operations we have $E^G_i = c$, (because updates span all the CGs). With these estimates and using Eq. \ref{eq:cost}, we have the following cost function:
\begin{align}
cost =  w.(\frac{T.L}{B} + \frac{T}{B.c}\sum\limits_{i=0}^{L}g_i) + 
        \sum \limits_{i=0}^Lp_i.g_i + \nonumber \\
        q. \sum \limits_{i=0}^L \frac{s_i}{B.g_i} + 
        u. \sum \limits_{i=0}^L \frac{T}{B} \nonumber
\end{align}
Here $p_i$ is the number of point queries at level $i$, and can be estimated using a probability distribution that captures the third assumption. For example, value of $p_i$ can be treated as an exponential distribution, where as the level $i$ increases, the chances of a point query at that level decreases exponentially. After removing the terms independent of $g_i$, we get the following optimization problem:
\begin{align}
    \label{eq:opt1}
    \forall i: 0 \leq i \leq L \\
    cost_i(g_i) := \frac{w.T.g_i}{B.c} + p_i.g_i + \frac{q.s_i}{B.g_i} \nonumber \\ 
    s.t.: \qquad    1 \leq g_i \leq c \nonumber \\
    g^*_i = \arg\!\min_{g_i}\, cost_i(g_i) \nonumber
\end{align}
We solve the above optimization problem for each level individually to get the number of CGs $g_i$ for each level $i$. Since we estimate $E^G_i$ and $E^g_i$ based on the sizes of the projection, instead of the projections themselves, the optimization function outputs the optimal CG sizes for each level, instead of the exact CG configuration. To get the exact CG configuration at each level, we can uniformly split $c$ columns into $g_i$ column-groups.

\textit{Scenario 2:} In this scenario, we relax the assumptions of scenario 1 and instead collect more statistics about the workload. Specifically, we compute the median projection size at each level, for each operation. We denote them by $r^P_i$, $r^Q_i$, and $r^U_i$ as projection sizes for \emph{read}, \emph{scan}, and \emph{update} operations respectively.
%In the previous scenario, the drawback is that if a workload does not comply with the assumptions then the best column-group configuration that it provides will be far from optimal.  
Due to the lack of any information about which columns exactly constitute the specific column-groups and projections, we assume that columns in projections uniformly span across all the column-groups. Under that assumption, the number of column-groups required to answer a projection can be given by $\left\lceil r^*_i / \cgsz_i \right\rceil$. Therefore, we have the following:
\begin{align}
    \text{for read operation} \qquad &E^g_i := \left\lceil \frac{r^P_i} {\cgsz_i} \right\rceil \nonumber \\
    \text{for scan operation} \qquad &E^G_i := \left\lceil \frac{r^Q_i} {\cgsz_i} \right\rceil \cdot cg\_size_i \nonumber \\
    \text{for update operation} \qquad &E^G_i := \left\lceil \frac{r^U_i} {\cgsz_i} \right\rceil \cdot cg\_size_i \nonumber 
\end{align}
Using $\cgsz_i = c/g_i$, we get the following cost function:
\begin{align}
cost =  w.(\frac{T.L}{B} + \frac{T}{B.c}\sum\limits_{i=0}^{L}g_i) + 
        \sum \limits_{i=0}^Lp_i.\left\lceil \frac{r^P_i.g_i} {c} \right\rceil  + \nonumber \\
        q. \sum \limits_{i=0}^L \frac{s_i}{g_i.B}.\left\lceil \frac{r^Q_i.g_i} {c} \right\rceil  + 
        u. \sum \limits_{i=0}^L \frac{T}{g_i.B}.\left\lceil \frac{r^U_i.g_i} {c} \right\rceil \nonumber
\end{align}
Similar to scenario 1, $p_i$ is the number of point queries at level $i$, and its value can be either estimated using a probability distribution or by collecting per level statistics. After removing the terms independent of $g_i$, we get the following optimization problem: 
\begin{align}
    \label{eq:opt2}
    \forall i &: 0 \leq i \leq L \\
    cost_i(g_i) &:=  \frac{w.T.g_i}{B.c} + 
                    p_i.\left\lceil \frac{r^P_i.g_i} {c} \right\rceil + \nonumber \\
                    & \frac{q.s_i}{g_i.B}.\left\lceil \frac{r^Q_i.g_i} {c} \right\rceil + 
                    \frac{u.T}{g_i.B}.\left\lceil \frac{r^U_i.g_i} {c} \right\rceil \nonumber \\ 
    s.t. &: \qquad    1 \leq g_i \leq c \nonumber \\
    g^*_i &= \arg\!\min_{g_i}\, cost_i(g_i) \nonumber
\end{align}
Similar to scenario 1, we pick the best $g_i$ at each level, and to get the exact CG configuration at each level, we uniformly split $c$ columns into $g_i$ column-groups.
